# Supplementary material for: Current density functional framework for spin-orbit coupling: Extension to periodic systems
Source: arXiv:2403.14420 source file (2024-03-21)
Supplement: Supplementary file 1 [file Supplementary-Material.pdf]

**Supplementary Material for “Current density functional framework for spin–orbit coupling: Extension to periodic systems”**

Yannick J. Franzke<sup>1</sup> and Christof Holzer<sup>2</sup>

<sup>1</sup>*Otto Schott Institute of Materials Research, Friedrich Schiller University Jena,  
Löbdergraben 32, 07743 Jena, Germany*

<sup>2</sup>*Institute of Theoretical Solid State Physics, Karlsruhe Institute of Technology (KIT),  
Wolfgang-Gaede-Straße 1, 76131 Karlsruhe, Germany*

(\*Email for correspondence: christof.holzer@kit.edu)

(\*Email for correspondence: yannick.franzke@uni-jena.de)

(Dated: 21 March 2024)

## CONTENTS

|                                                                       |    |
|-----------------------------------------------------------------------|----|
| <b>I. Linear One-Dimensional Pt Chain</b>                             | 3  |
| A. Computational Details and Detailed Results                         | 3  |
| <b>II. Two-Dimensional Transition-Metal Dichalcogenide Monolayers</b> | 5  |
| A. Computational Details                                              | 5  |
| B. Results                                                            | 6  |
| <b>III. Three-Dimensional Silver Halide Crystals</b>                  | 10 |
| A. Computational Details                                              | 10 |
| B. Results                                                            | 11 |
| <b>References</b>                                                     | 14 |

# I. LINEAR ONE-DIMENSIONAL PT CHAIN

## A. Computational Details and Detailed Results

Two Pt atoms are placed in a unit cell with a cell parameter  $d$ . Relativistic effects are introduced through small-core Dirac–Fock effective core potentials (ECP-60).<sup>1</sup> The dhf-SVP-2c orbital and auxiliary basis sets are applied<sup>2</sup> and large integration grids<sup>3,4</sup> (grid size 4) are employed for the numerical integration of the exchange-correlation potential<sup>5</sup> with the TPSS functional.<sup>6</sup> Note that the ripser module uses the resolution of the identity approximation (RI- $J$ ) in combination with the continuous fast multipole method (CFMM).<sup>7,8</sup> Default settings are employed for RI- $J$ , CFMM, and the transformation to the orthogonal basis set for the diagonalization of the Kohn–Sham or Fock matrix.<sup>8,9</sup> A Gaussian smearing of 0.01 Hartree is applied<sup>10</sup> and a  $k$ -mesh of 32 points is used. The self-consistent field (SCF) procedure is converged with a threshold of  $10^{-8}$  Hartree. Kramers-restricted (KR) and Kramers-unrestricted (KU) calculations are started from a molecular extended Hückel guess with a closed-shell configuration and an open-shell configuration using four unpaired electrons, respectively. For the KU calculations, the initial wavefunction is chosen to be an eigenfunction of the spin operator  $\hat{S}_x$ . Periodicity is also assumed along the  $x$  direction.<sup>9</sup> Structures in TURBOMOLE format<sup>9,11–15</sup> are available from Ref. 16. Results are listed in Tab. I. Here, the CDFT energies are always lower than the DFT energy, i.e. a more negative energy is found.

TABLE I. Total SCF energies in Hartree obtained with the 2c KR DFT, 2c KU DFT, 2c KR CDFT, and 2c KU CDFT approach, and energies for the limit of a vanishing Gaussian smearing (limit). The expectation values of spin  $S_x$  are listed for the open-shell calculations. The TPSS functional<sup>6</sup> is employed with the dhf-SVP-2c basis set<sup>2</sup> and a Dirac–Fock ECP for Pt.<sup>1</sup> 2c DFT results are taken from Ref. 16.

| $d$ | KR DFT limit | KR DFT    | KR CDFT limit | KR CDFT   | KU DFT limit | KU DFT    | KU DFT $\langle S_x \rangle$ | KU CDFT limit | KU CDFT   | KU CDFT $\langle S_x \rangle$ |
|-----|--------------|-----------|---------------|-----------|--------------|-----------|------------------------------|---------------|-----------|-------------------------------|
| 4.0 | -239.0074    | -239.0065 | -239.0077     | -239.0067 | -239.0074    | -239.0065 | $3.62 \times 10^{-5}$        | -239.0076     | -239.0067 | $2.64 \times 10^{-8}$         |
| 4.1 | -239.0592    | -239.0580 | -239.0594     | -239.0583 | -239.0592    | -239.0580 | $2.35 \times 10^{-5}$        | -239.0594     | -239.0583 | $-1.00 \times 10^{-14}$       |
| 4.2 | -239.0975    | -239.0961 | -239.0977     | -239.0963 | -239.0975    | -239.0961 | $4.72 \times 10^{-5}$        | -239.0977     | -239.0963 | $1.00 \times 10^{-14}$        |
| 4.3 | -239.1251    | -239.1234 | -239.1254     | -239.1237 | -239.1251    | -239.1234 | $3.41 \times 10^{-4}$        | -239.1253     | -239.1236 | $2.08 \times 10^{-4}$         |
| 4.4 | -239.1443    | -239.1423 | -239.1446     | -239.1425 | -239.1443    | -239.1423 | $4.77 \times 10^{-4}$        | -239.1446     | -239.1425 | $7.00 \times 10^{-14}$        |
| 4.5 | -239.1568    | -239.1544 | -239.1571     | -239.1547 | -239.1568    | -239.1544 | $5.10 \times 10^{-4}$        | -239.1570     | -239.1546 | $1.69 \times 10^{-3}$         |
| 4.6 | -239.1641    | -239.1613 | -239.1644     | -239.1616 | -239.1641    | -239.1613 | $5.05 \times 10^{-4}$        | -239.1643     | -239.1615 | $3.40 \times 10^{-3}$         |
| 4.7 | -239.1672    | -239.1640 | -239.1675     | -239.1643 | -239.1672    | -239.1640 | $3.94 \times 10^{-4}$        | -239.1675     | -239.1642 | $5.12 \times 10^{-3}$         |
| 4.8 | -239.1672    | -239.1636 | -239.1675     | -239.1639 | -239.1672    | -239.1636 | $3.97 \times 10^{-3}$        | -239.1675     | -239.1638 | $3.72 \times 10^{-2}$         |
| 4.9 | -239.1648    | -239.1607 | -239.1651     | -239.1610 | -239.1650    | -239.1611 | $2.54 \times 10^{-1}$        | -239.1656     | -239.1618 | $3.81 \times 10^{-1}$         |
| 5.0 | -239.1606    | -239.1560 | -239.1609     | -239.1564 | -239.1614    | -239.1575 | $4.91 \times 10^{-1}$        | -239.1621     | -239.1583 | $5.62 \times 10^{-1}$         |
| 5.1 | -239.1550    | -239.1501 | -239.1554     | -239.1504 | -239.1565    | -239.1525 | $6.27 \times 10^{-1}$        | -239.1573     | -239.1534 | $6.78 \times 10^{-1}$         |
| 5.2 | -239.1486    | -239.1432 | -239.1489     | -239.1436 | -239.1506    | -239.1464 | $7.13 \times 10^{-1}$        | -239.1515     | -239.1474 | $7.59 \times 10^{-1}$         |
| 5.3 | -239.1415    | -239.1357 | -239.1418     | -239.1361 | -239.1439    | -239.1395 | $7.76 \times 10^{-1}$        | -239.1449     | -239.1406 | $8.18 \times 10^{-1}$         |
| 5.4 | -239.1340    | -239.1278 | -239.1343     | -239.1282 | -239.1367    | -239.1320 | $8.30 \times 10^{-1}$        | -239.1379     | -239.1332 | $8.76 \times 10^{-1}$         |
| 5.5 | -239.1262    | -239.1197 | -239.1266     | -239.1201 | -239.1293    | -239.1241 | $8.84 \times 10^{-1}$        | -239.1306     | -239.1256 | $9.39 \times 10^{-1}$         |
| 5.6 | -239.1183    | -239.1115 | -239.1187     | -239.1118 | -239.1217    | -239.1162 | $9.27 \times 10^{-1}$        | -239.1232     | -239.1179 | $9.98 \times 10^{-1}$         |
| 5.7 | -239.1104    | -239.1032 | -239.1108     | -239.1036 | -239.1141    | -239.1083 | $9.69 \times 10^{-1}$        | -239.1159     | -239.1104 | 1.05                          |
| 5.8 | -239.1025    | -239.0950 | -239.1029     | -239.0954 | -239.1067    | -239.1006 | 1.00                         | -239.1087     | -239.1030 | 1.09                          |
| 5.9 | -239.0948    | -239.0869 | -239.0952     | -239.0873 | -239.0994    | -239.0931 | 1.03                         | -239.1017     | -239.0958 | 1.11                          |
| 6.0 | -239.0873    | -239.0791 | -239.0877     | -239.0795 | -239.0924    | -239.0859 | 1.04                         | -239.0948     | -239.0887 | 1.13                          |

## II. TWO-DIMENSIONAL TRANSITION-METAL DICHALCOGENIDE MONOLAYERS

### A. Computational Details

Band gaps and Rashba splittings are calculated for the transition-metal dichalcogenide monolayers MoS<sub>2</sub>, MoSe<sub>2</sub>, MoTe<sub>2</sub>, WS<sub>2</sub>, WSe<sub>2</sub>, and WTe<sub>2</sub> with the PBE,<sup>17</sup> M06-L,<sup>18</sup> r<sup>2</sup>SCAN,<sup>19,20</sup> TASK,<sup>21</sup> TPSS,<sup>6</sup> Tao–Mo,<sup>22</sup> and PKZB<sup>23</sup> density functional approximations (DFAs). Note that we use Libxc<sup>24–26</sup> for M06-L, r<sup>2</sup>SCAN, TASK, Tao–Mo, and PKZB. The dhf-TZVP-2c orbital and auxiliary basis sets are applied.<sup>2</sup> Originally, the dhf-type basis sets only employ ECPs for elements beyond Kr. That is, Dirac–Fock ECPs are employed for Mo (ECP-28), W (ECP-60), and Te (ECP-28).<sup>1,27,28</sup> However, this leads to rather large deviations from the relativistic all-electron calculations at the PBE level for MoSe<sub>2</sub> and WSe<sub>2</sub>.<sup>29,30</sup> See Tabs. II and III. Therefore, we applied a small-core Dirac–Fock ECP for Se (ECP-10) as well.<sup>27,31</sup> The corresponding results are shown in Tabs. IV and V.

Large integration grids<sup>3,4</sup> (grid size 3) are employed for the numerical integration of the exchange-correlation potential.<sup>5</sup> Again, default settings are applied for RI-*J*, CFMM, and the transformation to the orthogonal basis set for the diagonalization of the Kohn–Sham or Fock matrix.<sup>8,9</sup> The SCF procedure is converged with a threshold of  $10^{-7}$  Hartree and a *k*-mesh of  $33 \times 33$  points is used. Structures are taken from Ref. 29.

## B. Results

TABLE II. Band gaps and Rashba splittings of the valence band at the K point for transition-metal dichalcogenide monolayers at the 1c DFT, 2c DFT, and 2c CDFT level with the dhf-TZVP-2c basis set and DF-ECPs for Mo and Te. All values in eV.

| System            | DFA                 | Band Gap |        |         | Rashba Splitting |         |
|-------------------|---------------------|----------|--------|---------|------------------|---------|
|                   |                     | 1c DFT   | 2c DFT | 2c CDFT | 2c DFT           | 2c CDFT |
| MoS <sub>2</sub>  | PBE                 | 1.827    | 1.757  | 1.755   | 0.102            | 0.102   |
|                   | M06-L               | 1.814    | 1.772  | 1.772   | 0.107            | 0.112   |
|                   | r <sup>2</sup> SCAN | 1.940    | 1.884  | 1.879   | 0.103            | 0.116   |
|                   | TASK                | 2.035    | 1.979  | 1.968   | 0.105            | 0.130   |
|                   | TPSS                | 1.829    | 1.775  | 1.774   | 0.102            | 0.106   |
|                   | Tao-Mo              | 1.828    | 1.774  | 1.773   | 0.101            | 0.104   |
|                   | PKZB                | 1.829    | 1.775  | 1.774   | 0.101            | 0.103   |
| MoSe <sub>2</sub> | PBE                 | 1.560    | 1.504  | 1.504   | 0.102            | 0.102   |
|                   | M06-L               | 1.567    | 1.509  | 1.508   | 0.107            | 0.113   |
|                   | r <sup>2</sup> SCAN | 1.658    | 1.602  | 1.596   | 0.104            | 0.119   |
|                   | TASK                | 1.738    | 1.681  | 1.669   | 0.107            | 0.135   |
|                   | TPSS                | 1.566    | 1.510  | 1.508   | 0.103            | 0.107   |
|                   | Tao-Mo              | 1.564    | 1.508  | 1.508   | 0.102            | 0.105   |
|                   | PKZB                | 1.562    | 1.506  | 1.506   | 0.102            | 0.104   |
| MoTe <sub>2</sub> | PBE                 | 1.157    | 1.039  | 1.039   | 0.185            | 0.185   |
|                   | M06-L               | 1.182    | 1.060  | 1.053   | 0.192            | 0.209   |
|                   | r <sup>2</sup> SCAN | 1.235    | 1.116  | 1.101   | 0.186            | 0.218   |
|                   | TASK                | 1.287    | 1.161  | 1.126   | 0.197            | 0.269   |
|                   | TPSS                | 1.170    | 1.051  | 1.048   | 0.185            | 0.195   |
|                   | Tao-Mo              | 1.168    | 1.051  | 1.049   | 0.185            | 0.188   |
|                   | PKZB                | 1.160    | 1.042  | 1.042   | 0.186            | 0.189   |

TABLE III. Band gaps and Rashba splittings of the valence band at the K point for transition-metal dichalcogenide monolayers at the 1c DFT, 2c DFT, and 2c CDFT level with the dhf-TZVP-2c basis set and DF-ECPs for W and Te. All values in eV.

| System           | DFA                 | Band Gap |        |         | Rashba Splitting |         |
|------------------|---------------------|----------|--------|---------|------------------|---------|
|                  |                     | 1c DFT   | 2c DFT | 2c CDFT | 2c DFT           | 2c CDFT |
| WS <sub>2</sub>  | PBE                 | 1.999    | 1.697  | 1.697   | 0.343            | 0.343   |
|                  | M06-L               | 2.024    | 1.803  | 1.798   | 0.357            | 0.369   |
|                  | r <sup>2</sup> SCAN | 2.156    | 1.868  | 1.845   | 0.351            | 0.379   |
|                  | TASK                | 2.261    | 2.037  | 2.006   | 0.364            | 0.416   |
|                  | TPSS                | 2.031    | 1.758  | 1.752   | 0.343            | 0.351   |
|                  | Tao-Mo              | 2.040    | 1.754  | 1.749   | 0.337            | 0.343   |
|                  | PKZB                | 2.023    | 1.752  | 1.750   | 0.339            | 0.342   |
| WSe <sub>2</sub> | PBE                 | 1.654    | 1.385  | 1.385   | 0.354            | 0.354   |
|                  | M06-L               | 1.676    | 1.447  | 1.440   | 0.366            | 0.381   |
|                  | r <sup>2</sup> SCAN | 1.782    | 1.534  | 1.507   | 0.363            | 0.395   |
|                  | TASK                | 1.872    | 1.637  | 1.610   | 0.378            | 0.440   |
|                  | TPSS                | 1.672    | 1.436  | 1.429   | 0.353            | 0.362   |
|                  | Tao-Mo              | 1.680    | 1.433  | 1.427   | 0.347            | 0.354   |
|                  | PKZB                | 1.664    | 1.435  | 1.433   | 0.350            | 0.353   |
| WTe <sub>2</sub> | PBE                 | 1.219    | 0.933  | 0.933   | 0.423            | 0.423   |
|                  | M06-L               | 1.253    | 0.968  | 0.957   | 0.431            | 0.456   |
|                  | r <sup>2</sup> SCAN | 1.325    | 1.039  | 1.005   | 0.436            | 0.483   |
|                  | TASK                | 1.388    | 1.096  | 1.050   | 0.465            | 0.566   |
|                  | TPSS                | 1.237    | 0.960  | 0.954   | 0.422            | 0.435   |
|                  | Tao-Mo              | 1.241    | 0.963  | 0.957   | 0.419            | 0.426   |
|                  | PKZB                | 1.227    | 0.953  | 0.951   | 0.423            | 0.427   |

TABLE IV. Band gaps and Rashba splittings of the valence band at the K point for transition-metal dichalcogenide monolayers at the 1c DFT, 2c DFT, and 2c CDFT level with the dhf-TZVP-2c basis set and DF-ECPs for Mo, Se, and Te. All values in eV.

| System            | DFA                 | Band Gap |        |         | Rashba Splitting |         |
|-------------------|---------------------|----------|--------|---------|------------------|---------|
|                   |                     | 1c DFT   | 2c DFT | 2c CDFT | 2c DFT           | 2c CDFT |
| MoS <sub>2</sub>  | PBE                 | 1.827    | 1.757  | 1.755   | 0.102            | 0.102   |
|                   | M06-L               | 1.814    | 1.772  | 1.772   | 0.107            | 0.112   |
|                   | r <sup>2</sup> SCAN | 1.940    | 1.884  | 1.879   | 0.103            | 0.116   |
|                   | TASK                | 2.035    | 1.979  | 1.968   | 0.105            | 0.130   |
|                   | TPSS                | 1.829    | 1.775  | 1.774   | 0.102            | 0.106   |
|                   | Tao-Mo              | 1.828    | 1.774  | 1.773   | 0.101            | 0.104   |
|                   | PKZB                | 1.829    | 1.775  | 1.774   | 0.101            | 0.103   |
| MoSe <sub>2</sub> | PBE                 | 1.554    | 1.453  | –       | 0.166            | –       |
|                   | PKZB                | 1.558    | 1.455  | 1.455   | 0.166            | 0.169   |
|                   | Tao-Mo              | 1.561    | 1.459  | 1.458   | 0.166            | 0.170   |
|                   | TPSS                | 1.563    | 1.459  | 1.458   | 0.167            | 0.174   |
|                   | M06-L               | 1.563    | 1.460  | 1.455   | 0.170            | 0.181   |
|                   | r <sup>2</sup> SCAN | 1.657    | 1.554  | 1.544   | 0.166            | 0.189   |
|                   | TASK                | 1.735    | 1.629  | 1.607   | 0.172            | 0.218   |
| MoTe <sub>2</sub> | PBE                 | 1.157    | 1.039  | –       | 0.185            | –       |
|                   | PKZB                | 1.160    | 1.042  | 1.042   | 0.186            | 0.189   |
|                   | Tao-Mo              | 1.168    | 1.051  | 1.049   | 0.185            | 0.188   |
|                   | TPSS                | 1.170    | 1.051  | 1.048   | 0.185            | 0.195   |
|                   | M06-L               | 1.182    | 1.060  | 1.053   | 0.192            | 0.209   |
|                   | r <sup>2</sup> SCAN | 1.235    | 1.116  | 1.101   | 0.186            | 0.218   |
|                   | TASK                | 1.287    | 1.161  | 1.126   | 0.197            | 0.269   |

TABLE V. Band gaps and Rashba splittings of the valence band at the K point for transition-metal dichalcogenide monolayers at the 1c DFT, 2c DFT, and 2c CDFT level with the dhf-TZVP-2c basis set and DF-ECPs for W, Se, and Te. All values in eV.

| System           | DFA                 | Band Gap |        |         | Rashba Splitting |         |
|------------------|---------------------|----------|--------|---------|------------------|---------|
|                  |                     | 1c DFT   | 2c DFT | 2c CDFT | 2c DFT           | 2c CDFT |
| WS <sub>2</sub>  | PBE                 | 1.999    | 1.697  | 1.697   | 0.343            | 0.343   |
|                  | M06-L               | 2.024    | 1.803  | 1.798   | 0.357            | 0.369   |
|                  | r <sup>2</sup> SCAN | 2.156    | 1.868  | 1.845   | 0.351            | 0.379   |
|                  | TASK                | 2.261    | 2.037  | 2.006   | 0.364            | 0.416   |
|                  | TPSS                | 2.031    | 1.758  | 1.752   | 0.343            | 0.351   |
|                  | Tao-Mo              | 2.040    | 1.754  | 1.749   | 0.337            | 0.343   |
|                  | PKZB                | 2.023    | 1.752  | 1.750   | 0.339            | 0.342   |
| WSe <sub>2</sub> | PBE                 | 1.627    | 1.324  | –       | 0.409            | –       |
|                  | PKZB                | 1.652    | 1.377  | 1.374   | 0.407            | 0.410   |
|                  | Tao-Mo              | 1.667    | 1.371  | 1.367   | 0.403            | 0.411   |
|                  | TPSS                | 1.660    | 1.379  | 1.371   | 0.409            | 0.420   |
|                  | M06-L               | 1.668    | 1.413  | 1.405   | 0.422            | 0.440   |
|                  | r <sup>2</sup> SCAN | 1.774    | 1.482  | 1.452   | 0.419            | 0.457   |
|                  | TASK                | 1.867    | 1.604  | 1.571   | 0.440            | 0.514   |
| WTe <sub>2</sub> | PBE                 | 1.219    | 0.933  | –       | 0.423            | –       |
|                  | PKZB                | 1.227    | 0.953  | 0.951   | 0.423            | 0.427   |
|                  | Tao-Mo              | 1.241    | 0.963  | 0.957   | 0.419            | 0.426   |
|                  | TPSS                | 1.237    | 0.960  | 0.954   | 0.422            | 0.435   |
|                  | M06-L               | 1.253    | 0.968  | 0.957   | 0.431            | 0.456   |
|                  | r <sup>2</sup> SCAN | 1.325    | 1.039  | 1.005   | 0.436            | 0.483   |
|                  | TASK                | 1.388    | 1.096  | 1.050   | 0.465            | 0.566   |

### III. THREE-DIMENSIONAL SILVER HALIDE CRYSTALS

#### A. Computational Details

Silver halide systems are commonly studied with relativistic methods<sup>32–34</sup> and we have previously calculated the band gaps and cell structure with various meta-GGAs in DFT framework.<sup>16</sup> Thus, we complement these results with the CDFT treatment. Computational settings are chosen accordingly. That is, the dhf-SVP orbital and auxiliary basis sets<sup>2</sup> are applied with small-core Dirac–Fock ECPs (ECP-28) for Ag and I.<sup>35,36</sup> The TPSS,<sup>6</sup> revTPSS,<sup>37,38</sup> Tao–Mo,<sup>22</sup> PKZB,<sup>23</sup> r<sup>2</sup>SCAN,<sup>19,20</sup> and M06-L<sup>18</sup> density functional approximations are used with large integration grids (grid size 4).<sup>3,4</sup> We use Libxc<sup>24–26</sup> for revTPSS, Tao–Mo, PKZB and M06-L. The D3 dispersion correction is applied if available for the given DFA.<sup>39–43</sup> Default settings are chosen for RI-*J*, CFMM, and the transformation to the orthogonal basis set for the diagonalization of the Kohn–Sham or Fock matrix.<sup>8,9</sup> An SCF convergence threshold of  $10^{-7}$  Hartree is applied and a  $k$ -mesh of  $7 \times 7 \times 7$  point is employed. Cell structures are optimized with weight derivatives and an energy threshold of  $10^{-6}$  Hartree.<sup>44</sup> Results for AgCl, AgBr, and AgI are listed in Tabs. VI, VII, and VIII, respectively. Inclusion of the current density in the exchange-correlation potential is indicated by a “c” for the functional acronym. Initial cell structures were taken from Ref. 16.

## B. Results

TABLE VI. Optimized lattice constant  $a$  (in Å, rocksalt structure) of three-dimensional AgCl and band gaps (in eV) at high symmetry points of the first Brillouin zone with various density functional approximations and the dhf-SVP basis sets.<sup>2</sup> A Dirac–Fock ECP is applied for Ag (ECP-28).<sup>35</sup> A “c” indicates the current-dependent variant of the DFA. Results for DFAs without inclusion of the current density are taken from Ref. 16, except for M06-L. Calculations are performed without dispersion correction (no D3) and with the D3 correction using Becke–Johnson damping (D3-BJ).<sup>39,40</sup>

| DFA                  | Dispersion | $a$   | L–L   | $\Gamma$ – $\Gamma$ | X–X   | L– $\Gamma$ |
|----------------------|------------|-------|-------|---------------------|-------|-------------|
| TPSS                 | no D3      | 5.586 | 4.553 | 3.042               | 4.135 | 0.966       |
| cTPSS                | no D3      | 5.578 | 4.539 | 3.056               | 4.138 | 0.964       |
| revTPSS              | no D3      | 5.561 | 4.381 | 3.023               | 4.126 | 0.890       |
| crevTPSS             | no D3      | 5.542 | 4.350 | 3.059               | 4.135 | 0.885       |
| Tao–Mo               | no D3      | 5.541 | 4.242 | 3.099               | 4.238 | 0.971       |
| cTao–Mo              | no D3      | 5.518 | 4.212 | 3.150               | 4.251 | 0.971       |
| PKZB                 | no D3      | 5.636 | 4.593 | 3.099               | 4.259 | 1.176       |
| cPKZB                | no D3      | 5.644 | 4.604 | 3.086               | 4.256 | 1.178       |
| r <sup>2</sup> SCAN  | no D3      | 5.576 | 5.017 | 3.545               | 4.564 | 1.413       |
| cr <sup>2</sup> SCAN | no D3      | 5.564 | 5.001 | 3.570               | 4.569 | 1.413       |
| M06-L                | no D3      | 5.636 | 4.947 | 3.357               | 4.654 | 1.464       |
| cM06-L               | no D3      | 5.640 | 4.951 | 3.349               | 4.649 | 1.464       |
| TPSS                 | D3-BJ      | 5.498 | 4.400 | 3.213               | 4.175 | 0.943       |
| cTPSS                | D3-BJ      | 5.461 | 4.334 | 3.293               | 4.193 | 0.937       |
| revTPSS              | D3-BJ      | 5.476 | 4.233 | 3.204               | 4.169 | 0.873       |
| crevTPSS             | D3-BJ      | 5.445 | 4.179 | 3.274               | 4.184 | 0.870       |
| Tao–Mo               | D3-BJ      | 5.511 | 4.203 | 3.166               | 4.255 | 0.971       |
| cTao–Mo              | D3-BJ      | 5.499 | 4.186 | 3.194               | 4.262 | 0.972       |
| r <sup>2</sup> SCAN  | D3-BJ      | 5.517 | 4.943 | 3.677               | 4.592 | 1.416       |
| cr <sup>2</sup> SCAN | D3-BJ      | 5.514 | 4.939 | 3.683               | 4.592 | 1.416       |

TABLE VII. Optimized lattice constant  $a$  (in Å, rocksalt structure) of three-dimensional AgBr and band gaps (in eV) at high symmetry points of the first Brillouin zone with various density functional approximations and the dhf-SVP basis sets.<sup>2</sup> A Dirac–Fock ECP is applied for Ag (ECP-28).<sup>35</sup> A “c” indicates the current-dependent variant of the DFA. Results for DFAs without inclusion of the current density are taken from Ref. 16, except for M06-L. Calculations are performed without dispersion correction (no D3) and with the D3 correction using Becke–Johnson damping (D3-BJ).<sup>39,40</sup>

| DFA                  | Dispersion | $a$   | L–L   | $\Gamma$ – $\Gamma$ | X–X   | L– $\Gamma$ |
|----------------------|------------|-------|-------|---------------------|-------|-------------|
| TPSS                 | no D3      | 5.812 | 3.988 | 2.899               | 3.677 | 0.950       |
| cTPSS                | no D3      | 5.802 | 3.971 | 2.918               | 3.679 | 0.949       |
| revTPSS              | no D3      | 5.784 | 3.871 | 2.963               | 3.667 | 0.936       |
| crevTPSS             | no D3      | 5.764 | 3.839 | 2.999               | 3.672 | 0.936       |
| Tao–Mo               | no D3      | 5.738 | 3.781 | 3.140               | 3.792 | 1.079       |
| cTao–Mo              | no D3      | 5.736 | 3.779 | 3.143               | 3.792 | 1.079       |
| PKZB                 | no D3      | 5.868 | 4.128 | 2.985               | 3.812 | 1.189       |
| cPKZB                | no D3      | 5.875 | 4.138 | 2.973               | 3.812 | 1.190       |
| r <sup>2</sup> SCAN  | no D3      | 5.811 | 4.501 | 3.361               | 4.094 | 1.416       |
| cr <sup>2</sup> SCAN | no D3      | 5.800 | 4.486 | 3.384               | 4.095 | 1.418       |
| M06-L                | no D3      | 5.909 | 4.440 | 3.134               | 4.204 | 1.452       |
| cM06-L               | no D3      | 5.916 | 4.447 | 3.120               | 4.199 | 1.450       |
| TPSS                 | D3-BJ      | 5.708 | 3.815 | 3.092               | 3.708 | 0.951       |
| cTPSS                | D3-BJ      | 5.673 | 3.754 | 3.163               | 3.719 | 0.956       |
| revTPSS              | D3-BJ      | 5.690 | 3.715 | 3.143               | 3.695 | 0.942       |
| crevTPSS             | D3-BJ      | 5.655 | 3.653 | 3.218               | 3.707 | 0.948       |
| Tao–Mo               | D3-BJ      | 5.743 | 3.789 | 3.128               | 3.790 | 1.077       |
| cTao–Mo              | D3-BJ      | 5.731 | 3.771 | 3.155               | 3.794 | 1.080       |
| r <sup>2</sup> SCAN  | D3-BJ      | 5.774 | 4.448 | 3.444               | 4.104 | 1.423       |
| cr <sup>2</sup> SCAN | D3-BJ      | 5.758 | 4.429 | 3.473               | 4.107 | 1.426       |

TABLE VIII. Optimized lattice constant  $a$  (in Å, rocksalt structure) of three-dimensional AgI and band gaps (in eV) at high symmetry points of the first Brillouin zone with various density functional approximations and the dhf-SVP basis sets.<sup>2</sup> Dirac–Fock ECPs are applied for Ag (ECP-28) and I (ECP-28).<sup>35,36</sup> A “c” indicates the current-dependent variant of the DFA. Results for DFAs without inclusion of the current density are taken from Ref. 16, except for M06-L. Calculations are performed without dispersion correction (no D3) and with the D3 correction using Becke–Johnson damping (D3-BJ).<sup>39,40</sup>

| DFA                  | Dispersion | $a$   | L–L   | $\Gamma$ – $\Gamma$ | X–X   | L–X   |
|----------------------|------------|-------|-------|---------------------|-------|-------|
| TPSS                 | no D3      | 6.153 | 3.249 | 2.047               | 2.937 | 0.583 |
| cTPSS                | no D3      | 6.150 | 3.244 | 2.052               | 2.940 | 0.579 |
| revTPSS              | no D3      | 6.116 | 3.149 | 2.132               | 2.998 | 0.537 |
| crevTPSS             | no D3      | 6.098 | 3.122 | 2.161               | 3.014 | 0.512 |
| Tao–Mo               | no D3      | 6.071 | 3.099 | 2.343               | 3.108 | 0.616 |
| cTao–Mo              | no D3      | 6.069 | 3.086 | 2.339               | 3.109 | 0.619 |
| PKZB                 | no D3      | 6.200 | 3.409 | 2.153               | 2.987 | 0.826 |
| cPKZB                | no D3      | 6.210 | 3.422 | 2.138               | 2.979 | 0.839 |
| r <sup>2</sup> SCAN  | no D3      | 6.159 | 3.776 | 2.501               | 3.237 | 0.911 |
| cr <sup>2</sup> SCAN | no D3      | 6.156 | 3.772 | 2.504               | 3.240 | 0.907 |
| M06-L                | no D3      | 6.325 | 3.511 | 1.891               | 2.976 | 1.116 |
| cM06-L               | no D3      | 6.327 | 3.512 | 1.889               | 2.974 | 1.117 |
| TPSS                 | D3-BJ      | 5.982 | 2.988 | 2.352               | 3.098 | 0.343 |
| cTPSS                | D3-BJ      | 5.980 | 2.985 | 2.354               | 3.099 | 0.341 |
| revTPSS              | D3-BJ      | 5.949 | 2.883 | 2.443               | 3.156 | 0.291 |
| crevTPSS             | D3-BJ      | 5.952 | 2.889 | 2.435               | 3.152 | 0.296 |
| Tao–Mo               | D3-BJ      | 6.068 | 3.095 | 2.347               | 3.110 | 0.613 |
| cTao–Mo              | D3-BJ      | 6.062 | 3.087 | 2.358               | 3.116 | 0.604 |
| r <sup>2</sup> SCAN  | D3-BJ      | 6.156 | 3.773 | 2.506               | 3.240 | 0.907 |
| cr <sup>2</sup> SCAN | D3-BJ      | 6.155 | 3.771 | 2.506               | 3.241 | 0.905 |

## REFERENCES

- <sup>1</sup>D. Figgen, K. A. Peterson, M. Dolg, and H. Stoll, J. Chem. Phys. **130**, 164108 (2009).
- <sup>2</sup>F. Weigend and A. Baldes, J. Chem. Phys. **133**, 174102 (2010).
- <sup>3</sup>O. Treutler and R. Ahlrichs, J. Chem. Phys. **102**, 346 (1995).
- <sup>4</sup>O. Treutler, *Entwicklung und Anwendung von Dichtefunktionalmethoden*, Dissertation (Dr. rer. nat.), University of Karlsruhe (TH), Germany (1995).
- <sup>5</sup>A. M. Burow and M. Sierka, J. Chem. Theory Comput. **7**, 3097 (2011).
- <sup>6</sup>J. Tao, J. P. Perdew, V. N. Staroverov, and G. E. Scuseria, Phys. Rev. Lett. **91**, 146401 (2003).
- <sup>7</sup>A. M. Burow, M. Sierka, and F. Mohamed, J. Chem. Phys. **131**, 214101 (2009).
- <sup>8</sup>R. Łazarski, A. M. Burow, and M. Sierka, J. Chem. Theory Comput. **11**, 3029 (2015).
- <sup>9</sup>TURBOMOLE GmbH, (2024), manual of TURBOMOLE V7.8.1, a development of University of Karlsruhe and Forschungszentrum Karlsruhe GmbH, 1989-2007, TURBOMOLE GmbH, since 2007; available from <https://www.turbomole.org/turbomole/turbomole-documentation/> (retrieved March 4, 2024).
- <sup>10</sup>G. Kresse and J. Furthmüller, Comput. Mater. Sci. **6**, 15 (1996).
- <sup>11</sup>R. Ahlrichs, M. Bär, M. Häser, H. Horn, and C. Kölmel, Chem. Phys. Lett. **162**, 165 (1989).
- <sup>12</sup>F. Furche, R. Ahlrichs, C. Hättig, W. Klopper, M. Sierka, and F. Weigend, Wiley Interdiscip. Rev.: Comput. Mol. Sci. **4**, 91 (2014).
- <sup>13</sup>S. G. Balasubramani, G. P. Chen, S. Coriani, M. Diedenhofen, M. S. Frank, Y. J. Franzke, F. Furche, R. Grotjahn, M. E. Harding, C. Hättig, A. Hellweg, B. Helmich-Paris, C. Holzer, U. Huniar, M. Kaupp, A. Marefat Khah, S. Karbalaee Khani, T. Müller, F. Mack, B. D. Nguyen, S. M. Parker, E. Perlt, D. Rappoport, K. Reiter, S. Roy, M. Rückert, G. Schmitz, M. Sierka, E. Tapavicza, D. P. Tew, C. van Wüllen, V. K. Voora, F. Weigend, A. Wodyński, and J. M. Yu, J. Chem. Phys. **152**, 184107 (2020).
- <sup>14</sup>Y. J. Franzke, C. Holzer, J. H. Andersen, T. Begušić, F. Bruder, S. Coriani, F. Della Sala, E. Fabiano, D. A. Fedotov, S. Fürst, S. Gillhuber, R. Grotjahn, M. Kaupp, M. Kehry, M. Krstić, F. Mack, S. Majumdar, B. D. Nguyen, S. M. Parker, F. Pauly, A. Pausch, E. Perlt, G. S. Phun, A. Rajabi, D. Rappoport, B. Samal, T. Schrader, M. Sharma, E. Tapavicza, R. S. Treß, V. Voora, A. Wodyński, J. M. Yu, B. Zerulla, F. Furche, C. Hättig, M. Sierka, D. P. Tew, and F. Weigend, J. Chem. Theory Comput. **19**, 6859 (2023).

- <sup>15</sup>TURBOMOLE GmbH, (2024), developers' version of TURBOMOLE V7.8.1, a development of University of Karlsruhe and Forschungszentrum Karlsruhe GmbH, 1989-2007, TURBOMOLE GmbH, since 2007; available from <https://www.turbomole.org> (retrieved March 4, 2024).
- <sup>16</sup>Y. J. Franzke, W. M. Schosser, and F. Pauly, *Phys. Rev. B* (2024), 10.48550/arXiv.2305.03817, accepted.
- <sup>17</sup>J. P. Perdew, K. Burke, and M. Ernzerhof, *Phys. Rev. Lett.* **77**, 3865 (1996).
- <sup>18</sup>Y. Zhao and D. G. Truhlar, *J. Chem. Phys.* **125**, 194101 (2006).
- <sup>19</sup>J. W. Furness, A. D. Kaplan, J. Ning, J. P. Perdew, and J. Sun, *J. Phys. Chem. Lett.* **11**, 8208 (2020).
- <sup>20</sup>J. W. Furness, A. D. Kaplan, J. Ning, J. P. Perdew, and J. Sun, *J. Phys. Chem. Lett.* **11**, 9248 (2020).
- <sup>21</sup>T. Aschebrock and S. Kümmel, *Phys. Rev. Res.* **1**, 033082 (2019).
- <sup>22</sup>J. Tao and Y. Mo, *Phys. Rev. Lett.* **117**, 073001 (2016).
- <sup>23</sup>J. P. Perdew, S. Kurth, A. c. v. Zupan, and P. Blaha, *Phys. Rev. Lett.* **82**, 2544 (1999).
- <sup>24</sup>M. A. L. Marques, M. J. T. Oliveira, and T. Burnus, *Comput. Phys. Commun.* **183**, 2272 (2012).
- <sup>25</sup>S. Lehtola, C. Steigemann, M. J. T. Oliveira, and M. A. L. Marques, *SoftwareX* **7**, 1 (2018).
- <sup>26</sup>“Libxc,” Version 6.2.2, available from <https://www.tddft.org/programs/libxc/> (retrieved July 26, 2023).
- <sup>27</sup>K. A. Peterson, D. Figgen, E. Goll, H. Stoll, and M. Dolg, *J. Chem. Phys.* **119**, 11113 (2003).
- <sup>28</sup>K. A. Peterson, D. Figgen, M. Dolg, and H. Stoll, *J. Chem. Phys.* **126**, 124101 (2007).
- <sup>29</sup>P. Miró, M. Audiffred, and T. Heine, *Chem. Soc. Rev.* **43**, 6537 (2014).
- <sup>30</sup>M. Kadek, B. Wang, M. Joosten, W.-C. Chiu, F. Mairesse, M. Repisky, K. Ruud, and A. Bansil, *Phys. Rev. Mater.* **7**, 064001 (2023).
- <sup>31</sup>M. Dolg, Effective core potentials of Se (ECP10MDF) taken from <https://www.tc.uni-koeln.de/PP/clickpse.en.html> (retrieved March 19, 2024).
- <sup>32</sup>J. E. Peralta, J. Uddin, and G. E. Scuseria, *J. Chem. Phys.* **122**, 084108 (2005).
- <sup>33</sup>R. Zhao, Y. Zhang, Y. Xiao, and W. Liu, *J. Chem. Phys.* **144**, 044105 (2016).
- <sup>34</sup>M. Kadek, M. Repisky, and K. Ruud, *Phys. Rev. B* **99**, 205103 (2019).
- <sup>35</sup>D. Figgen, G. Rauhut, M. Dolg, and H. Stoll, *Chem. Phys.* **311**, 227 (2005).
- <sup>36</sup>K. A. Peterson, B. C. Shepler, D. Figgen, and H. Stoll, *J. Phys. Chem. A* **110**, 13877 (2006).
- <sup>37</sup>J. P. Perdew, A. Ruzsinszky, G. I. Csonka, L. A. Constantin, and J. Sun, *Phys. Rev. Lett.* **103**, 026403 (2009).

- <sup>38</sup>J. P. Perdew, A. Ruzsinszky, G. I. Csonka, L. A. Constantin, and J. Sun, Phys. Rev. Lett. **106**, 179902 (2011).
- <sup>39</sup>S. Grimme, J. Antony, S. Ehrlich, and H. Krieg, J. Chem. Phys. **132**, 154104 (2010).
- <sup>40</sup>S. Grimme, S. Ehrlich, and L. Goerigk, J. Comput. Chem. **32**, 1456 (2011).
- <sup>41</sup>L. Goerigk, A. Hansen, C. Bauer, S. Ehrlich, A. Najibi, and S. Grimme, Phys. Chem. Chem. Phys. **19**, 32184 (2017).
- <sup>42</sup>A. Patra, S. Jana, L. A. Constantin, and P. Samal, J. Chem. Phys. **153**, 084117 (2020).
- <sup>43</sup>S. Ehlert, U. Huniar, J. Ning, J. W. Furness, J. Sun, A. D. Kaplan, J. P. Perdew, and J. G. Brandenburg, J. Chem. Phys. **154**, 061101 (2021).
- <sup>44</sup>Minor deviations from the rocksalt structure were removed by symmetrization. This changed the energy by less than  $3 \cdot 10^{-4}$  Hartree or less than 1 kJ/mol. Typically, changes are below  $10^{-5}$  Hartree.
